# Supplementary material for: Towards a fully differentiable digital twin for solar cells
Source: arXiv:2512.02904 ancillary file (2025-12-02)
Supplement: Supplementary file 1 [file SI.pdf]

# Towards a fully differentiable digital twin for solar cells: Supporting Information

Marie Louise Schubert[1,2,†], Houssam Metni[1,2,†], Jan David Fischbach[1], Benedikt Zerulla[1], Marjan Krstić[14], Ulrich W. Paetzold[3,4], Seyedamir Orooji[3,4], Olivier J. J. Ronsin[7], Yasin Ameslon[7,8], Jens Harting[7,8,9], Thomas Kirchartz[10,11], Sandheep Ravishankar[10], Chris Dreessen[10], Eunchi Kim[10], Christian Sprau[4,5], Mohamed Hussein[4,6], Alexander Colsmann[4,5], Karen Forberich[7], Klaus Jäger[12,13], Pascal Friederich[1,2,⋆], and Carsten Rockstuhl[1,14,⋆]

[1]Institute of Nanotechnology, Karlsruhe Institute of Technology (KIT), Karlsruhe, Germany
[2]Institute of Theoretical Informatics, Karlsruhe Institute of Technology (KIT), Karlsruhe, Germany
[3]Institute of Microstructure Technology, Karlsruhe Institute of Technology (KIT), Karlsruhe, Germany
[4]Light Technology Institute, Karlsruhe Institute of Technology (KIT), Karlsruhe, Germany
[5]Material Research Center for Energy Systems, Karlsruhe Institute of Technology (KIT), Karlsruhe, Germany
[6]Department of Physics, Faculty of Science, Ain Shams University, Cairo, Egypt
[7]Helmholtz-Institute Erlangen-Nürnberg for Renewable Energy (IET-2), Forschungszentrum Jülich, Erlangen, Germany
[8]Department of Chemical and Biological Engineering, Friedrich-Alexander-Universität Erlangen-Nürnberg, Erlangen, Germany
[9]Department of Physics, Friedrich-Alexander-Universität Erlangen-Nürnberg (FAU), Erlangen, Germany
[10]IMD-3 Photovoltaik, Forschungszentrum Jülich (FZJ), Jülich, Germany
[11]Faculty of Electrical Engineering and Information Technology, University of Duisburg-Essen, Duisburg, Germany
[12]Department Optics for Solar Energy (SE-AOPT), Helmholtz-Zentrum Berlin für Materialien und Energie GmbH, Berlin, Germany
[13]Zuse Institute Berlin, Berlin, Germany
[14]Institute of Theoretical Solid State Physics, Karlsruhe Institute of Technology (KIT), Karlsruhe, Germany
[†]These authors contributed equally; marie.schubert@kit.edu and houssam.metni@kit.edu
[⋆]These authors are corresponding authors; pascal.friederich@kit.edu and carsten.rockstuhl@kit.edu

# 1 Details of the molecules

In this study, a thin film of photoactive material was selected made from crystalline domains of acceptor molecule (2,2'-((2Z,2'Z)-((12,13-bis(2-ethylhexyl)-3,9-diundecyl-12,13-dihydro-[1,2,5]thiadiazolo[3,4-e]thieno[2,"3":4',5']thieno[2',3':4,5]pyrrolo[3,2-g]thieno[2',3':4,5]thieno[3,2-b]indole-2,10-diyl)bis
(methanylylidene))bis(5,6-difluoro-3-oxo-2,3-dihydro-1H-indene-2,1-diylidene))dimalononitrile) (in short, **Y6**) dispersed within Poly[(2,6-(4,8-bis(5-(2-ethylhexyl-3-fluoro)thiophen-2-yl)-benzo[1,2-b:4,5-b']dithiophene))-alt-(5,5-(1',3'-di-2-thienyl-5',7'-bis(2-ethylhexyl)benzo[1',2'-c:4',5'-c']dithiophene-4,8-dione)] (in short, **PM6**) polymer. The PM6:Y6 molecular mixture is known as an excellent organic photoactive material, here embedded into an overall stack architecture as presented as shown in Figure 2 b) of the manuscript.
For the PM6:Y6 system, structural properties of the molecular models were defined separately. The PM6 polymer was represented by two monomer molecules with lattice constants of 3.98, 0.44 and 2.28 nm. The crystalline Y6 was modeled with lattice constants of 1.51, 2.89 and 2.01 nm.

# 2 Morphology

## 2.1 Phase field model

### 2.1.1 Simulation Parameters

The inputs required by the morphology part of our digital twin are material properties and the film processing conditions. The details of those are given in Table 1.

| Parameter | Unit | Value for PM6 | Value for Y6 |
|---|---|---|---|
| Density | kg/m$^3$ | 1100 | 1320 |
| Molar mass | kg/mol | 0.21 | 1.45 |
| Energy barrier upon crystallization | kJ/kg | $7.6 \cdot 10^4$ | $5 \cdot 10^4$ |
| Heat of fusion | kJ/kg | $5 \cdot 10^4$ | $4 \cdot 10^4$ |
| Melting temperature | K | 673 | 571 |
| Amorphous-amorphous interaction parameter | — | 1 | 1 |
| Crystalline-amorphous interaction parameter | — | 0.1 | 0.1 |
| Crystal mobility coefficient in the longitudinal direction | s$^{-1}$ | $1.5 \cdot 10^{-11}$ | 15 |
| Longitudinal/transversal growth ratio | — | 10 | 10 |
| Processing temperature | K | 333 | 333 |

Table 1: Phase field simulation parameters used for the calculation of PM6:Y6 volume fractions and crystalline order parameters presented in the manuscript.

### 2.1.2 Gibbs free energy

Three different free energy density variation contributions are used to describe the amorphous-amorphous phase transition ($\Delta G_v^{am}$), the amorphous-crystalline phase transition ($\Delta G_v^{cr}$), and the gas phase free energy density change upon gases mixing ($\Delta G_v^{gas}$) of a mixture of $n$ components.

**Amorphous-amorphous phase transition** The free energy density variation $\Delta G_v^{am}$ variation due to the amorphous-amorphous phase transition is

$$\Delta G_v^{am} = \frac{RT}{v_0}\left((1-p(\phi_{gas}))\sum_{i=1}^{n}\varphi_i\frac{ln(\varphi_i)}{N_i} + (1-p(\phi_{gas}))\sum_{i=1}^{n}\sum_{j>i}^{n}\varphi_i\varphi_j\chi_{ij,aa} + \sum_{i=1}^{n}\frac{\kappa_i}{2}(\nabla\varphi_i)^2\right) \quad (1)$$

$\sum_{i=1}^{n}\varphi_i\frac{ln(\varphi_i)}{N_i}$ are the entropy terms of mixing, where $\varphi_i$ and $N_i$ are the volume fraction and molar size of component $i$, respectively. $\sum_{i=1}^{n}\sum_{j>i}^{n}\varphi_i\varphi_j\chi_{ij,aa}$ are energetic terms due to the interaction between pairs of amorphous components, where $\varphi_j$ is the volume fraction of component $j$ and $\chi_{ij,aa}$ is the binary amorphous-amorphous interaction parameter between component $i$ and component $j$. $\sum_{i=1}^{n}\frac{\kappa_i}{2}(\nabla\varphi_i)^2$ is an interfacial energy term, where $\kappa_i$ is a surface tension parameter related to the

gradients of volume fraction. $R$, $T$, and $v_0$ are the ideal gas constant, temperature and the smallest component molar volume, respectively. The bulk terms of the free energy are interpolated between the condensed phase and the gas phase using the interpolation function $p\left(\phi_{gas}\right) = {\phi_{gas}}^2(3 - 2\phi_{gas})$, where $\phi_{gas}$ is the order parameter representing the phase transition between condensed matter and the gas state.

**Amorphous-crystalline phase transition** The free energy density variation $\Delta {G_v}^{cr}$ due to the crystallization of $n_{crys}$ components is

$$\begin{aligned}\Delta {G_v}^{cr} = \sum_{i=1}^{n_{crys}} \Bigg[ &(1 - p(\phi_{gas}))\, \rho_i\, {\varphi_i}^2 \Big( g(\phi_i) W_i + p(\phi_i) L_i \Big( \frac{T}{T_{m,i}} - 1 \Big) \Big) \\ &+ (1 - p(\phi_{gas})) \frac{RT}{v_0} \sum_{j \neq i}^{n} \Big( {\phi_i}^2 \varphi_i \varphi_j \chi_{ij,ca} + \phi_i \phi_j \varphi_i \varphi_j \chi_{ij,cc} \Big) \\ &+ \frac{1}{2} {\varepsilon_i}^2 (\nabla \phi_i)^2 + p(\phi_i) \frac{\pi}{2} \varepsilon_{g,i} \left| \nabla \right| \delta(\nabla \theta_i) + E_i {\phi_i}^2 {\phi_{gas}}^2 \Bigg]\end{aligned} \tag{2}$$

where $\rho_i {\varphi_i}^2 \left( g\left(\phi_i\right) W_i + p\left(\phi_i\right) L_i \left( \frac{T}{T_{m,i}} - 1 \right) \right)$ is the free energy gain upon crystallization of component $i$, with density $\rho_i$. Therein, $g\left(\phi_i\right) W_i$ is the energy barrier to crystallization of component $i$, where $g\left(\phi_i\right) = {\phi_i}^2 \left(\phi_i - 1\right)^2$ is a double well function depending on the crystalline order parameter $\phi_i$ of component $\phi_i$ and $W_i$ the height of the energy barrier. $p\left(\phi_i\right) L_i \left( \frac{T}{T_{m,i}} - 1 \right)$ is the driving force of crystallization, interpolated between an amorphous phase and a crystalline phase, with the interpolation function $p\left(\phi_i\right) = {\phi_i}^2(3 - 2\phi_i)$, where $L_i$ and $T_{m,i}$ are the heat of fusion and melting temperature of component $i$. $\frac{RT}{v_0} \sum_{j \neq i}^{n} {\phi_i}^2 \varphi_i \varphi_j \chi_{ij,ca}$ in Equation 2 is an energetic contribution due to interaction between crystalline/amorphous components pairs, where $\chi_{ij,ca}$ is the binary amorphous-crystalline interaction parameter. Similarly, $\frac{RT}{v_0} \sum_{j \neq i}^{n} \phi_i \phi_j \varphi_i \varphi_j \chi_{ij,cc}$ is an energetic contribution due to interaction between crystalline/crystalline components pairs, where $\chi_{ij,cc}$ is the binary crystalline-crystalline interaction parameter .$\frac{1}{2} {\varepsilon_i}^2 (\nabla\ \phi_i)^2$ and $p(\phi_i) \frac{\pi}{2} \varepsilon_{g,i} \left| \nabla \right| \delta(\nabla \theta_i)$ are surface energy contributions, where $\varepsilon_i$ and $\varepsilon_{g,i}$ are the surface tension parameters related to the gradients of order parameter and crystal orientation $\theta_i$ of crystals of component $i$. $E_i {\phi_i}^2 {\phi_{gas}}^2$ is a crystal-gas interaction to avoid the overlap between the crystalline and the gas phases that could occur due to the presence of diffuse interfaces that are characteristic of phase field simulations, where $E_i$ is a crystal-gas energy contribution. This contribution prevents the occurrence of nonphysical crystal instability. The bulk terms of the free energy are interpolated between the condensed phase and the gas phase using the interpolation function $p\left(\phi_{gas}\right)$.

**Mixing of evaporated liquids** Upon condensed-gas phase transition during solvent evaporation, gases form and stay in a mixed phase. The free energy density variation upon mixing of ideal gases $\Delta G_v^{gas}$ reads

$$\begin{aligned}\Delta G_v^{gas} &= p(\phi_{gas}) \frac{RT}{v_0} \sum_{i=1}^{n} \varphi_i \ln \left( \frac{P_i}{{P_i}^{sat}} \right) + \frac{\varepsilon_{gas}^2}{2} \left(\nabla \phi_{gas}\right)^2 \\ &= p(\phi_{gas}) \frac{RT}{v_0} \sum_{i=1}^{n} \varphi_i \ln \left( \frac{\varphi_i}{{\varphi_i}^{sat}} \right) + \frac{\varepsilon_{gas}^2}{2} \left(\nabla \phi_{gas}\right)^2\end{aligned} \tag{3}$$

$\sum_{i=1}^{n} \varphi_i \ln \left( \frac{\varphi_i}{{\varphi_i}^{sat}} \right)$ is an entropic term where we define $\varphi_i = \frac{P_i}{P_0}$ and ${\varphi_i}^{sat} = \frac{{P_i}^{sat}}{P_0}$. $P_i$, ${P_i}^{sat}$, and $P_0$ are the partial pressure, the vapor pressure of the gas $i$, and a reference pressure, respectively. The gases are assumed to have the same molecular size $N_i = 1$. $\frac{{\varepsilon_{gas}}^2}{2} \nabla(\phi_{gas})^2$ is a surface energy contribution, where $\varepsilon_{gas}$ is a surface tension parameter related to gradients of the order parameter representing the phase transition between condensed matter and gas state $\phi_{gas}$. The bulk term of the free energy is interpolated between the condensed phase and the gas phase using the interpolation function $p\left(\phi_{gas}\right)$.

**Total free energy** The total free energy $\Delta G$ expression is

$$\Delta G = \int_V dV(\Delta G_v{}^{am} + \Delta G_v{}^{cr} + \Delta G_v{}^{gas} + k\sum_{i=1}^{n} \varphi_i{}^{-1}) \tag{4}$$

where $k\sum_{i=1}^{n} \varphi_i{}^{-1}$ is a non-physical term added for numerical stability purposes, where $k$ is chosen small enough to avoid any impact on the simulated physics.

### 2.1.3 Kinetic equations coupled to fluid mechanics

The system's evolution towards equilibrium is calculated using Cahn-Hilliard (see Equation 5) and Allen-Cahn (see Equation 6 and Equation 8) equations, whereby the free energy is minimized at each time step. Fluid mechanics is coupled to these equations to include advective mass transport.

**Mass transport** The mass transport kinetics are governed by the Cahn-Hilliard-Cook equation, which allows us to determine the time evolution of the volume fraction for the first $i = 1 \ldots\ n-1$ components

$$\frac{\partial \varphi_i}{\partial t} + v\nabla\varphi_i = \frac{v_0}{RT}\nabla\left[\sum_{j=1}^{n-1} \Lambda_{ij}\nabla\left(\frac{\delta\Delta G}{\delta\varphi_j} - \frac{\delta\Delta G}{\delta\varphi_n}\right)\right] + \zeta_{CH}{}^{i} \tag{5}$$

where $v$, $\Lambda_{ij}$, and $\zeta_{CH}{}^{i}$ are a single velocity field, the field dependent Onsager mobility coefficients, and a Gaussian noise on the volume fraction to recover the effect of thermal fluctuations, respectively. The last volume fraction is deduced from the volume conservation law $\sum \varphi_i = 1$.

**Evaporation** The evaporation kinetics are governed by the advective Allen-Cahn equation on the evaporation order parameter

$$\frac{\partial \phi_{gas}}{\partial t} + v\nabla\phi_{gas} = -\frac{v_0}{RT} M_{gas}\frac{\delta\Delta G}{\delta\phi_{gas}} \tag{6}$$

where $M_{gas}$ is the Allen-Cahn mobility of the gas phase. An evaporation flux $j_{i,gas}$ is applied at the top boundary of the simulation box

$$j_{i,gas} = \alpha\sqrt{\frac{v_0}{2\pi RT}\frac{N_i}{\rho_i}} P_0(\varphi_i{}^{gas} - \varphi_i{}^{\infty}) \tag{7}$$

where $\varphi_i{}^{gas}$ is the volume fraction of component $i$ in the gas phase at the condensed-gas interface and $\varphi_i{}^{\infty}$ is defined such that $\varphi_i{}^{\infty} = \frac{P_i{}^{\infty}}{P_0}$, where $P_i{}^{\infty}$ is the partial pressure in the environment. The evaporation occurs in two steps: the first one being the formation of a gas film at the condensed phase surface, and the second one being the diffusion of the gas in the environment. Moreover, the evaporating solvents leaving the simulation box due to the evaporating flux are replaced by air to preserve the volume conservation required for the Cahn-Hilliard kinetics. The Flory-Huggins interaction parameter of the air with all the components is set to zero, and the vapor pressure is very high compared to the other components to minimize the presence of air in the liquid film due to the diffuse nature of interfaces in the phase field model.

**Crystallization** The crystallization kinetics are governed by the advective Allen-Cahn equation on the crystalline order parameter

$$\frac{\partial \phi_i}{\partial t} + v\nabla\phi_i = -\frac{v_0}{RT} M_i\frac{\delta\Delta G}{\delta\phi_i} + \zeta_{AC}{}^{i}, \tag{8}$$

where $M_i$ is the Allen-Cahn mobility of crystal $i$ and $\zeta_{AC}{}^{i}$ is a Gaussian noise on the order parameter to recover the effect of thermal fluctuations responsible for nucleation.

**Fluid flows** The Allen-Cahn and Cahn-Hilliard kinetic equations are used to determine the system's evolution towards equilibrium at each time step. Fluid mechanics equations are coupled to the kinetic equations to incorporate advective mass transport to the model. The fluid mechanics equations are derived assuming the system fluids to be incompressible. Mass is conserved, and buoyancy as well as gravitational forces are negligible as compared to capillary forces. In the limit of low Reynolds numbers (negligible inertia), we get

$$\nabla v = 0 \tag{9}$$

$$-\nabla P + \nabla\left(2\eta_{mix}S\right) + F_{\varphi} + F_{\phi} = 0 \tag{10}$$

where $v$ is the velocity, $P$ is the pressure, $S$ is the strain rate tensor, $\eta_{mix} = \prod_{i=1}^{n} {\eta_i}^{\varphi_i}$ is the viscosity of the liquid mixture, with $\eta_i$ the viscosity in the pure amorphous component $i$. In the crystal phase (vapor phase, respectively), the viscosity is set to a significantly higher value (significantly lower value). $F_{\varphi}$ and $F_{\phi}$ are capillary forces at the volume fraction and order parameter interfaces, respectively.

$$F_{\varphi} = \nabla\left[\sum_{i=1}^{n} \kappa_i(\left|\nabla\varphi_i\right|^2 I - \nabla\varphi_i \times \nabla\varphi_i)\right] \tag{11}$$

$$F_{\varphi} = \nabla\left[\sum_{i=1}^{n_{crys}} {\varepsilon_i}^2\left(\left|\nabla\phi_i\right|^2 I - \nabla\phi_i \times \nabla\phi_i\right) + {\varepsilon_{gas}}^2(\left|\nabla\phi_{gas}\right|^2 I - \nabla\phi_{gas} \times \nabla\phi_{gas})\right] \tag{12}$$

## 2.2 Morphology-aware electronic properties of organic solar cells

Once the active layer morphology is obtained, four morphology-aware descriptors allowing to evaluate the impact of the morphology on the electronic properties of the absorber layer [1, 2, 3, 4], will additionally be calculated in future works, building on an approach proposed previously [5, 6]. The first descriptor evaluates the efficiency of exciton dissociation into collectible free charge carriers, that is to say, the probability that an exciton dissociates into free charge carriers that are able to finally reach the desired electrodes. The second descriptor evaluates the impact of the solar cell morphology on non-geminate recombination. The third and fourth descriptors evaluate the impact of the morphology on electron and hole mobilities, respectively. These four morphology-aware descriptors will be passed to the electrical module of the digital twin in order to use morphology-dependent input parameters in drift-diffusion simulations, thus allowing the calculation of morphology-dependent current density-voltage ($JV$) curves.

# 3 Optics

For the PM6:Y6 system, structural properties of the molecular models were defined separately. The PM6 polymer was represented by two monomer molecules with lattice constants of 3.98, 0.44, and 2.28 nm. The crystalline Y6 was modeled with lattice constants of 1.51, 2.89, and 2.01 nm. Using the defined finite-size molecular models, the damped dynamic electric-electric, electric-magnetic and magnetic-magnetic polarizability tensors were calculated with TD-DFT. These dynamic polarizabilities are then used to construct the T-matrix, describing the light-matter interaction at the molecular level [7, 8]. The individual steps are described in the following.

## 3.1 The details of DFT calculations

The ground state electronic structure and properties were calculated using the development version of the quantum chemistry electronic structure code TURBOMOLE[9, 10] and density functional theory (DFT) method. In the case of the PM6 polymer, two monomers were stitched together as a molecular model and a full gradient-minimizing optimization technique was employed to obtain the final structure before moving further to the calculation of the excited state properties. In molecular optimization, the hybrid PBE0 DFT functional[11, 12] was used together with triple-$\zeta$-quality basis set with additional valence and polarization functions (def2-TZVP) [13, 14, 15, 16]. In further optical properties calculations of the donor material PM6, a coulomb-attenuated long-range-corrected hybrid cam-B3LYP functional [17] was employed in combination with the same def2-TZVP basis set. This functional was selected to properly account for long-range effects and charge-transfer states that exist within the polymer material incorporated in organic solar cells.

In the case of crystalline Y6 acceptor material, a hybrid TPSSh density exchange-correlation (XC) functional[18, 19, 20] was utilized. This choice was rationalized by the fact that Y6 forms a J-aggregate type of arrangement that is known to have low-energy lying excitations states. Thus, the TPSSh functional would better capture positions of those excitations in comparison to the cam-B3LYP XC functional, which is known to artificially blue-shift the predicted spectra. For the excited state calculations, the same atomic orbital (AO) basis set was used as in the case of PM6. In the case of Y6 crystalline material, a single point calculation was performed (without re-optimizing the structure) for the ground state electron density and energy, followed by a time-dependent DFT (TD-DFT) calculation for the dynamic polarizabilities.

The dynamic polarizability tensors were calculated for a set of complex frequencies covering the range from 300-1200 nm with a 2 nm step. The Lorentzian line-shape broadening (damping) factor was set to 0.1 eV as full-width-at-half-maximum (FWHM). The obtained dynamic polarizabilities were used to visualize absorption spectra and construct T-matrices for Maxwell scattering simulations as described previously. The absorption spectra in atomic units are determined as a trace of the imaginary part of 3x3 electric-electric dynamic polarizability:

$$A^{\omega} = \frac{1}{3}\,\mathrm{tr}[(\Im(\alpha^{\omega}_{ee})], \tag{13}$$

where $A$ denotes absorbance, $\omega$ is a frequency, and $ee$ indicates electric-electric components of the calculated polarizability tensors in atomic units. Finally, the spectra are normalized for direct comparison with measured spectra of the molecular thin films.

To obtain results as fast as possible and to reduce computational complexity in all calculations, resolution-of-identity (RI)[21] and multipole-accelerated RI (marij)[22] algorithms were additionally utilized. The same def2-TZVP basis set was used as an auxiliary basis set[13, 14, 15, 16]. Furthermore, a semi-numerical approach to calculate the exchange part (senex) of the DFT functional was employed to further economize the calculations, making them computationally very efficient[23].

All DFT and TD-DFT calculations were deposited in the NOMAD database and can be accessed under the following link: (`https://doi.org/10.17172/NOMAD/2025.11.20-2`)

## 3.2 Finite-size models of PM6 and Y6 molecular materials

In order to address the optical properties of the photoactive organic PM6:Y6 film within the solar cell stack, we need to calculate the optical response of building components on the quantum level. Due to the unknown morphological complexity of the PM6:Y6 thin film, we decided to use simplified molecular models for quantum calculations. Instead of describing a mixture of both molecules in our calculations, we opted for treating them separately to make the obtained properties of interest in a streamlined fashion. Thus, two separated molecular models were constructed and used as a basis for density functional theory calculations.

First, an acceptor crystalline molecular material of Y6 was considered. It was possible to obtain an already existing crystalline structure from the supplementary material of Ref. [24], which we used as a starting structural morphology in our calculations. A single monoclinic unit cell of Y6 material is composed of 8 molecules having in total 1016 atoms and unit cell vectors $a$ = 1.511 17 nm, $b$ = 5.7812 nm and $c$ = 2.0076 nm with angles between them $\alpha = \gamma = 90°$ and $\beta = 95.923°$ [24]. Molecules within have simplified Y6 structure with shortened C-side chains from $C_{11}H_{23}$ to $CH_3$. This is justifiable due to the fact that such long chains improve the solubility of organic molecules and usually do not play a role in the optical properties of organic dyes. To minimize computational demand on the quantum level and produce a molecular model with all three unit vectors of similar dimensions, we further reduced the unit cell to half length along vector $b$. Having all three vectors of the molecular model of similar lengths helps to reduce Rayleigh sphere overlap in Maxwell simulations, reducing artificial interactions with neighboring molecules of the periodic cell and obtaining spurious optical response. In total, this model has 4 simplified molecules of Y6 in a crystalline arrangement and 508 atoms as presented in **Figure 1**(a,b), below. In order to better distinguish each of the 4 molecules in the crystalline orientation, we colored each molecule with different colors in Figure 1(c,d).

Second, we consider a PM6 polymer in the context of molecular modeling and quantum chemistry calculations. For this polymer, there is no available starting structure. Thus, we build the smallest "polymer" molecular model of two identical monomer molecules of PM6 connected by a single covalent C-C bond. The second monomer is rotated by 180° around the backbone of the polymer

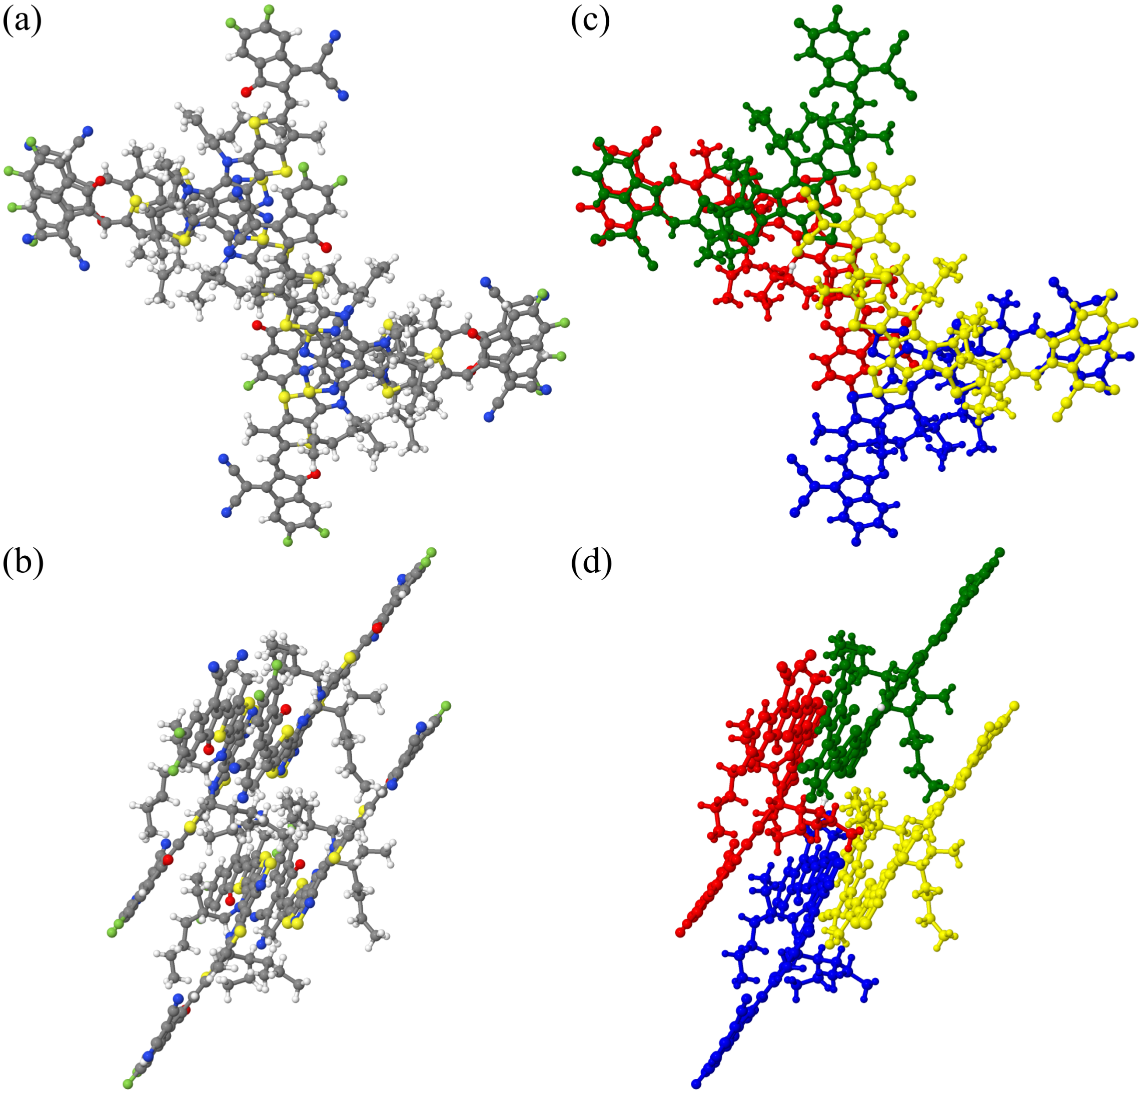


Figure 1: **(a)** A view along -x–direction of the molecular model containing 4 molecules of Y6 in crystalline arrangement. The balls in colors white, gray, blue, red, yellow, and green represent H, C, N, O, S, and F atoms, respectively. **(b)** A side-view along +y-direction of molecular model containing 4 molecules of Y6 in crystalline arrangement. **(c)** The same view as in (a), but with each of the 4 molecules color-marked. **(d)** The same view as in (b), but with the 4 molecules color-marked.

chain. The total molecular model has 314 atoms. The full geometry optimization in ground state was performed, and the obtained final structure has atom positions as depicted in **Figure 2**(a). In Figure 2(b), each monomer unit is visualized with a different color.

### 3.3 Optical properties of molecular models

The calculated complex dynamic polarizabilities within the spectral window of interest from the ultraviolet (UV) to infrared (IR) parts of the electromagnetic spectrum (EM) contain all necessary information to determine, for example, absorption of molecular materials among many other electronic optical properties. This can be achieved by applying Equation 13 given in Section 3.1 to TD-DFT calculated dynamic polarizabilities. The resulting spectra for both PM6 and Y6 molecular models are presented in **Figure 3**.

The absorbance of the PM6 simplified polymer molecular model (blue line in Figure 3) exhibits absorption in the UV and the visible part of the EM spectrum. The highest absorption is around 600 nm with two additionally pronounced peaks at above 500 nm and below 400 nm. In the case

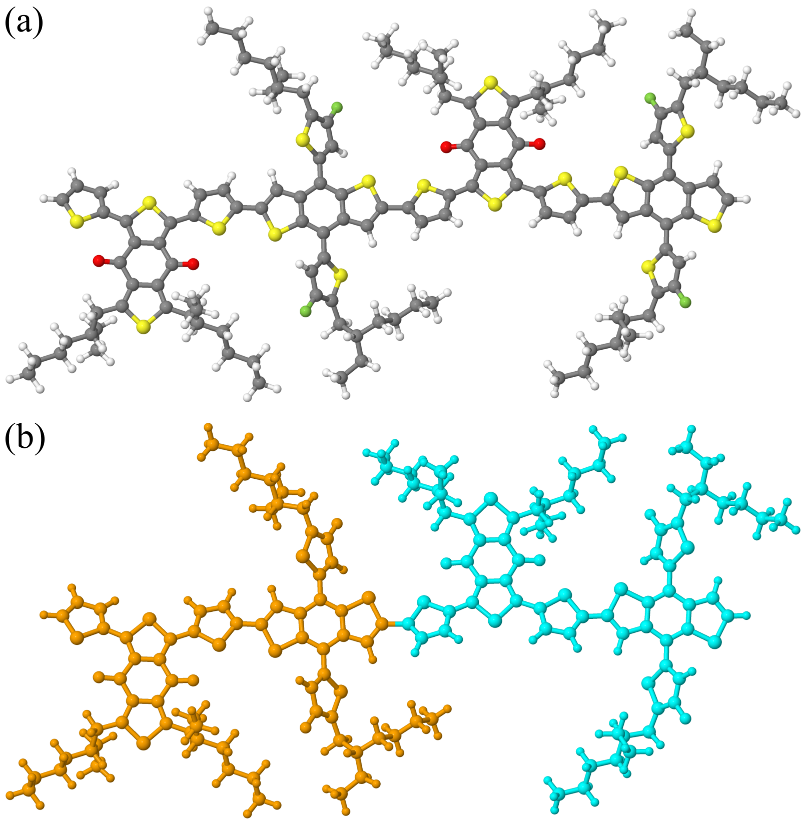


Figure 2: **(a)** The side-view of DFT optimized PM6 polymer model structure. White, gray, blue, red, yellow, and green balls represent H, C, N, O, S, and F atoms, respectively. **(b)** The same view as in (a) with the two individual monomers being color-marked.

of Y6 crystalline molecular material TD-DFT calculated spectrum (red line in Figure 3), the absorption maximum is close to 800 nm in the IR part of the spectrum with a side band at around 700 nm. Three additional lower intensity peaks are located above 550 nm, at around 500 nm and at about 400 nm. Remarkably, all predicted spectral features are recognizable in the experimentally reported spectra of thin films of these molecular materials by Yuan *et al.* in Figure 1.(E) of Ref. [25]. This fact gives us confirmation that our chosen molecular models are large enough to correctly obtain the optical response of materials on larger scales and confidence to proceed to the construction of T-matrices to fuel the Maxwell scattering simulations of a mixture of these two materials forming a thin film in the complete solar cell stack.

## 3.4 Relationship between dynamic polarizability tensors and T-matrices

In short, 6x6 dynamic complex dipolar polarizability tensors $\boldsymbol{\alpha}_{\nu\nu'}$ of molecular materials can be calculated using quantum chemistry methods such as TD-DFT, among others. These matrices are presented in Cartesian coordinates. In order to be able to incorporate molecular materials within Maxwell simulations of devices, in this case the solar cell stack, one needs to cross the bridge between the molecular (quantum) level and device (classical) level. Here, the dipolar transition matrix (T-matrix) comes in play, defined in the helicity basis as:

$$\mathbf{T} = \begin{pmatrix} \mathbf{T}_{\mathrm{NN}} & \mathbf{T}_{\mathrm{NM}} \\ \mathbf{T}_{\mathrm{MN}} & \mathbf{T}_{\mathrm{MM}} \end{pmatrix} = \frac{\mathrm{i}c_{\mathrm{h}} Z_{\mathrm{h}} k_{\mathrm{h}}^3}{6\pi} \begin{pmatrix} \mathbf{C}\left(\boldsymbol{\alpha}_{\mathrm{ee}}\right)\mathbf{C}^{-1} & \mathbf{C}\left(-\mathrm{i}\boldsymbol{\alpha}_{\mathrm{em}}/Z_{\mathrm{h}}\right)\mathbf{C}^{-1} \\ \mathbf{C}\left(\mathrm{i}\boldsymbol{\alpha}_{\mathrm{me}}/c_{\mathrm{h}}\right)\mathbf{C}^{-1} & \mathbf{C}\left(\boldsymbol{\alpha}_{\mathrm{mm}}/(c_{\mathrm{h}}Z_{\mathrm{h}})\right)\mathbf{C}^{-1} \end{pmatrix}, \tag{14}$$

where $\mathbf{C}$ is a unitary matrix converting a (polarizability) tensor from the Cartesian basis to the spherical basis, $c_{\mathrm{h}} = 1/\sqrt{\varepsilon_{\mathrm{h}}\mu_{\mathrm{h}}}$ is the speed of light in the surrounding medium, and $Z_{\mathrm{h}} = \sqrt{\mu_{\mathrm{h}}/\varepsilon_{\mathrm{h}}}$ is the wave impedance [26]. We emphasize that the $\boldsymbol{\alpha}_{\nu\nu'}$ are 3x3 complex matrices (tensors), allowing for anisotropic responses of the molecule(s). The subscript *ee* denotes the electric-electric

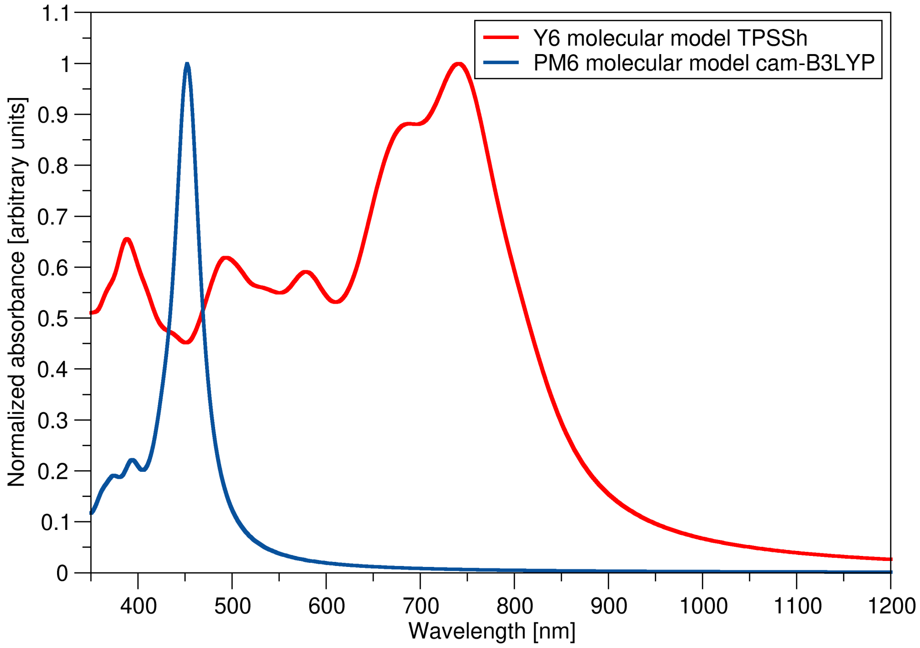


Figure 3: Normalized plots of TD-DFT calculated absorption spectra of PM6 and Y6 molecular models reproduce reported experimental spectra of PM6 and Y6 thin films in Figure 1.(E) of Ref. [25].

tensor, *em* is electric-magnetic, *me* is magnetic-electric, and *mm* are magnetic-magnetic interaction components of the polarizability tensor. All physical quantities are frequency-dependent in nature. Further details of this relationship can be found in the work from Fernandez-Corbaton *et al.*[26].

## 3.5 Homogenization

Homogenization computes the effective T-matrix ($\mathbf{T}_{\text{eff}}$) for bulk material by using the T-matrix of individual molecular units for constructing the collective response of complex structures. This multi-scale approach derives material parameters of an effective medium based on the constitutive relations. The effective T-matrix $\mathbf{T}_{\text{eff}}$ was computed using the treams framework [27]. The $\mathbf{T}_{\text{eff}}$ consolidates all non-local effects into an effectively local description, where the response of a unit cell is independent of neighboring unit cells, assuming plane wave illumination. It is given in a multi-polar basis and remains valid for all wave vector directions, without explicit dependence on any specific direction. This calculation was performed separately for PM6 and Y6. The effective T-matrix $\mathbf{T}_{\text{eff}}$ serves as a basis for determining key material parameters, such as permittivity $\boldsymbol{\varepsilon}_{\text{eff}}$ and permeability $\boldsymbol{\mu}_{\text{eff}}$. They are typically extracted using a linear $6 \times 6$ local bi-anisotropic model, relating electric displacement $\mathbf{D}$ and magnetic flux density $\mathbf{B}$ to the electric field $\mathbf{E}$ and magnetic field $\mathbf{H}$ in the frequency domain. The bi-anisotropic constitutive relations and the dipolar components of $\mathbf{T}_{\text{eff}}$ are bijectively linked. If the non-dipolar contributions of $\mathbf{T}_{\text{eff}}$ are negligible - often the case after accounting for all lattice interactions - the effective material parameters can be directly derived from $\mathbf{T}_{\text{eff}}$. Unlike other homogenization approaches, this method does not need any prior knowledge about the shape of the bulk material [8].

## 3.6 Calculation of Generation Rate

From $\mathbf{T}_{\text{eff}}$, the permittivities $\boldsymbol{\varepsilon}_{\text{eff}}$ of each material can be deduced. For the active material blend of the solar cell, a mass blend ratio of 1:1.2 is chosen between PM6 and Y6 [28, 29]. The effective permittivity of the PM6:Y6 blend was calculated by weighting the permittivities of Y6 and PM6 accordingly. The resulting optical constants n and k are compared to experimental data from Ref. [28] in **Figure 4**. In the further analysis, known permittivity values were used for the other, additional materials comprising the device architecture.
Optical solvers are needed to analyze the light propagation in the overall bulk material of the

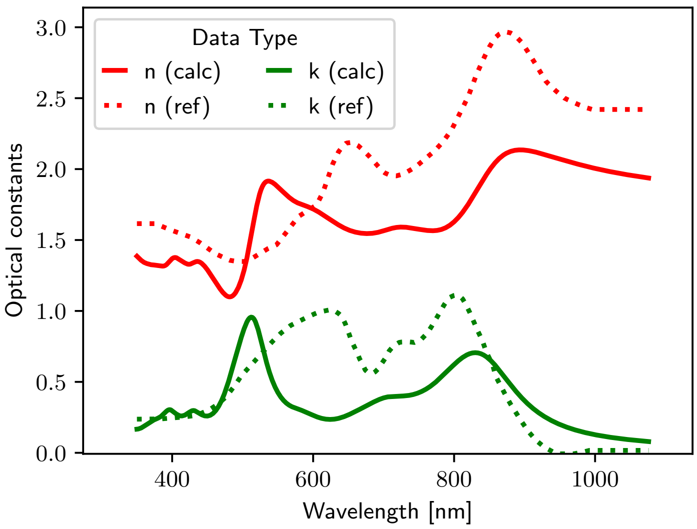


Figure 4: Optical constants of PM6:Y6 calculated with our methods, compared to Figure S5 (a) in Ref. [28].

solar cell. Depending on the complexity of a given problem, either numerical optical simulations or analytical methods can be used.

With the purpose of having a minimal digital twin model, we use a semi-analytical stack solver based on scattering matrices (S-matrices) [30] to study the optical response. The individual S-matrices of the layers and interfaces are analytically known (Fresnel coefficients). These can be cascaded using the Redhaffer star product [31]. Separating the stack into two S-matrices — one before and one after a certain interface of interest — one easily finds the excitation coefficients at that interface under illumination from the outside. What remains is to propagate the fields into the adjacent homogeneous layer to retrieve the spatially resolved absorption as $P_{\text{abs}}(x) = -0.5\omega\, |\text{E}(x)|^2\, \text{Im}(\varepsilon)$. With absorption $P_{\text{abs}}(x)$ we then calculate the generation rate $G$ as

$$G = \text{e} \int_x \int_\lambda P_{\text{abs}}(x)\, f(\lambda)\, \text{d}\lambda\, \text{d}x. \tag{15}$$

with e the elementary charge and the factor $f(\lambda)$ is defined as $f(\lambda) = \text{Irr}(\lambda)\, \frac{P_{\text{in}}}{A_{\text{in}}}$, where Irr is the irradiance at wavelength $\lambda$ based on the standard AM 1.5 spectrum and $P_{\text{in}}$ is the power input per area $A_{\text{in}}$. Equation 15 holds under the assumption that the internal quantum efficiency is 100 %. This implies that all absorbed photons in the photoactive layer are converted into free charge carriers.

## 3.7 Machine Learning based surrogate modeling

In order to enable a differentiable modeling of the generation rate (i.e., the output of the optics module), a neural network was trained to predict the generation rate as a function of the wavelength, incident angle, and photoactive material thickness. For this purpose, training data was generated by calculating the generation rate over the following ranges:

$$\theta \in [0^\circ, 89^\circ], \quad \lambda \in [300\,\text{nm},\, 1200\,\text{nm}], \quad d \in [100\,\text{nm},\, 300\,\text{nm}]$$

where $\theta$ is the incident angle, $\lambda$ the wavelength, and $d$ the thickness of the active material.

To approximate the generation rates as a differentiable function of the photoactive material layer thickness, a fully connected neural network was constructed. The model receives a single input feature—the photoactive material thickness—and outputs a two-dimensional grid of generation rates spanning a predefined grid of wavelengths and incident angles, defined based on the previous intervals. Specifically, the network maps the scalar input to a $(90 \times 901)$ output array, corresponding to 90 incident angles (from $0^\circ$ to $89^\circ$) and 901 wavelengths (from 300 nm to 1200 nm). The architecture consists of two hidden layers with 128 and 256 units, respectively, both followed by

ReLU activations. The final output layer is a dense layer with $90 \times 901 = 81090$ units, reshaped to form the predicted generation rate values.

The training of the model reached an $R^2$ accuracy of 0.99. **Figure 5** shows the evolution of the training loss over a few training epochs and the predicted vs. true generation rate values for the test set. **Figure 6** provides an example of predicted and true generation rates calculated for a photoactive material thickness of 190nm.

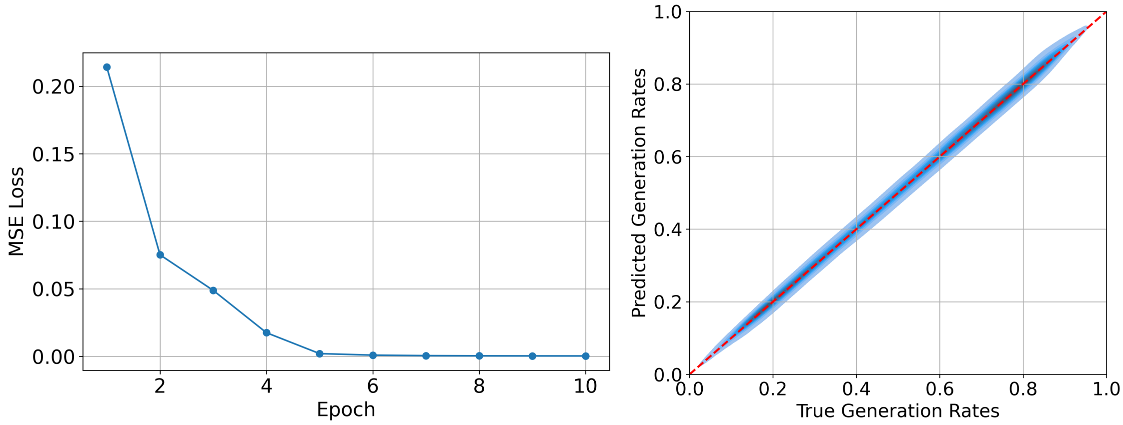


**(a)** Training loss evolution (over 10 epochs) **(b)** Predicted vs. true generation rate

Figure 5: (a) Evolution of the mean-squared-error training loss over the first 10 epochs. (b) Predicted vs. true generation rate values for the full test set (density plot).

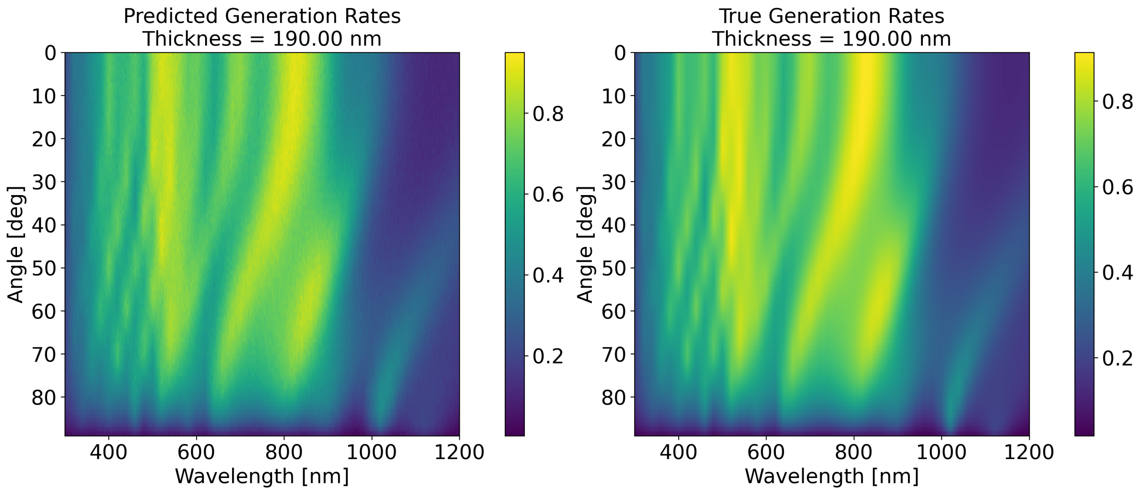


Figure 6: Example of two sets of generation rates calculated for an example photoactive material thickness of 190nm. On the left panel, the differentiable surrogate ML-based approximated generation rates (labeled as predicted), and on the right panel, the generation rates calculated using the classical non-differentiable module (labeled as true) are shown.

# 4 Electrical

## 4.1 Drift-Diffusion simulations

As mentioned in the main text, the software ASA numerically solves three coupled differential equations. The first equation is the Poisson equation

$$\frac{d^2\varphi}{dx^2} = \frac{-\rho(x)}{\varepsilon}, \tag{16}$$

where $\varphi$ is the electrostatic potential, $\epsilon$ is the permittivity, $\rho$ is the space charge density given by $\rho(x) = q(p(x) - n(x) + N_{\mathrm{D}}(x) - N_{\mathrm{A}}(x))$, $n$ and $p$ are the densities of electrons and holes, $N_{\mathrm{A}}$ is the density of ionized acceptor-like defects and $N_{\mathrm{D}}$ is the density of ionized donor-like defects. At steady state ($dn/dt = dp/dt = 0$), the continuity equations are given by

$$-\frac{1}{q}\frac{dJ_{\mathrm{n}}(x)}{dx} = -D_{\mathrm{n}}\frac{d^2n(x)}{dx^2} - F\mu_{\mathrm{n}}\frac{dn(x)}{dx} = G(x) - k_{\mathrm{rec}}\left(n(x)p(x) - n_{\mathrm{i}}^2\right) - \frac{\left(n(x)p(x) - n_{\mathrm{i}}^2\right)}{n(x)\tau_{\mathrm{p}} + p(x)\tau_{\mathrm{n}}}, \tag{17}$$

for electrons and

$$\frac{1}{q}\frac{dJ_{\mathrm{p}}(x)}{dx} = -D_{\mathrm{p}}\frac{d^2p(x)}{dx^2} + F\mu_{\mathrm{p}}\frac{dp(x)}{dx} = G(x) - k_{\mathrm{rec}}\left(n(x)p(x) - n_{\mathrm{i}}^2\right) - \frac{\left(n(x)p(x) - n_{\mathrm{i}}^2\right)}{n(x)\tau_{\mathrm{p}} + p(x)\tau_{\mathrm{n}}} \tag{18}$$

for holes. In Equations 17 and 18, $J_{\mathrm{n}}$ and $J_{\mathrm{p}}$ are the current densities of electrons and holes respectively, $D_{\mathrm{n,p}} = k_{\mathrm{B}}T \times \mu_{\mathrm{n,p}}$ are the diffusion coefficients for electrons and holes, $\mu_{\mathrm{n,p}}$ are the mobilities of electrons and holes, $k_{\mathrm{rec}}$ is the bimolecular recombination coefficient, $F = -d\varphi/dx$ is the electric field, $n_{\mathrm{i}}$ is the intrinsic carrier concentration and $\tau_{\mathrm{n}}$ and $\tau_{\mathrm{p}}$ are the Shockley-Read-Hall lifetimes of electrons and holes respectively. Equations 16 to 18 are numerically solved using the input parameters listed in Table 2 and suitable boundary conditions for each differential equation. No external series resistance was considered in the simulations. The one-sun generation rate was obtained from the optical simulations. For other light intensities, the one-sun generation rate was scaled using a corresponding constant factor. The temperature-dependent bimolecular recombination coefficient and mobilities were obtained by fitting the experimental data in ref.[32]. The cost function CF used was

$$CF = \sum_{j=1}^{m}\sum_{k=1}^{n}\left[\left(FF_{\mathrm{sim}}\left(I_{\mathrm{j}}, T_{\mathrm{k}}\right) + V_{\mathrm{oc,sim}}\left(I_{\mathrm{j}}, T_{\mathrm{k}}\right)\right) - \left(FF_{\mathrm{exp}}\left(I_{\mathrm{j}}, T_{\mathrm{k}}\right) + V_{\mathrm{oc,exp}}\left(I_{\mathrm{j}}, T_{\mathrm{k}}\right)\right)\right]^2, \tag{19}$$

where $I$ and $T$ are the sets of light intensity and temperature with $m$ and $n$ points respectively. The cost function is minimized to obtain the pre-factors and activation energies as explained in the main text.

| **Parameter** | **Unit** | **Cathode** | **Absorber** | **Anode** |
|---|---|---|---|---|
| Thickness | nm | | 100 [32] | |
| Relative permittivity | — | | 3.5 [33] | |
| Bandgap | eV | | 1.27 [33] | |
| Electron affinity | eV | | 4.1 [33] | |
| Effective density of states conduction band | $cm^{-3}$ | | $10^{20}$ [33] | |
| Effective density of states valence band | $cm^{-3}$ | | $10^{20}$ [33] | |
| Bimolecular recombination coefficient | $cm^3/s$ | | fitting parameter | |
| Non-radiative recombination lifetime | s | | $9.8 \cdot 10^{-6}$ [33] | |
| Electron mobility | $cm^2/Vs$ | | fitting parameter* | |
| Hole mobility | $cm^2/Vs$ | | fitting parameter* | |
| Doping density | $cm^{-3}$ | | 0 | |
| Injection barrier | meV | 50 | | 50 |
| Minority carrier surface recombination velocity | cm/s | $10^7$ | | $10^7$ |

Table 2: Drift-diffusion simulation parameters used to carry out the fits of the temperature and light intensity-dependent current-voltage curves of a PM6:Y6 solar cell. *The electron mobility was set equal to the hole mobility in the absorber.

## 4.2 Neural-Network surrogate modeling

A differentiable surrogate model was developed using a multi-output feedforward neural network to predict the $V_{oc}$ and $FF$. The network takes as input the temperature $T$ in $K$, the irradiance in $suns$, the layer thickness in $nm$, and outputs a two-dimensional vector corresponding to the predicted values of $V_{oc}$ and $FF$. The architecture consists of one shared hidden layer with 16 neurons and ReLU activation, followed by two separate branches—one for each target metric—each with a final dense layer producing a scalar output. Notably, each output path directly applies a ReLU activation to the shared hidden representation before a linear projection, resulting in a network with a total of two hidden layers per path (one shared and one implicit pre-output nonlinearity). The model is trained using the Adam optimizer with a learning rate of 0.01 and mean squared error as the loss function, over 100 epochs. **Figure 7** shows the evolution of training and validation losses across epochs, indicating good convergence and minimal overfitting. After training, the model's predictions on the test set are compared to the true experimental values. **Figure 8** illustrates the predicted versus true values for both $V_{oc}$ and $FF$, demonstrating high predictive accuracy and fidelity of the surrogate model.

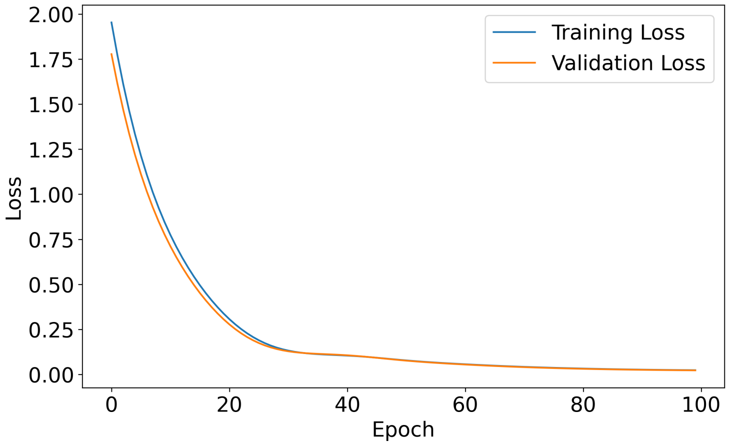


Figure 7: Training and validation loss over 100 epochs for the multi-output neural network.

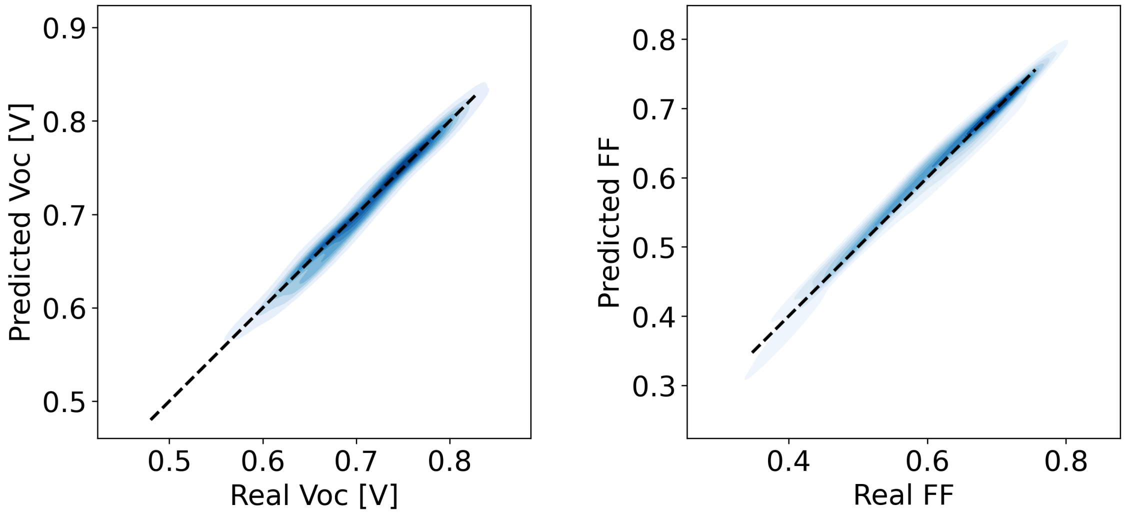


(a)

(b)

Figure 8: Predicted vs. real values for (a) $V_{oc}$ and (b) $FF$ on the test set.

# 5 Energy yield

## 5.1 EYCalc

Here, we provide a brief overview of the optics and electrics modules in the original version of the software EYCalc [34]. The optics module utilizes the transfer-matrix method to evaluate thin layers (coherent) and a series expansion based on the Beer-Lambert law for thick layers (incoherent). It calculates the reflectance, transmittance, and absorptance, resolved spectrally and angularly, for each layer in the stack. Additionally, the module supports simulations of stacks with textured surfaces through geometrical ray-tracing, as documented by Baker-Finch and McIntosh [35]. The electrics module determines the temperature-dependent $JV$ characteristics of the solar cells. It uses multiple diode parameters for each subcell, including the dark saturation current density, charge carrier collection efficiency, series resistance, and shunt resistance. To compute the $JV$ characteristics, the software offers two options: numerical calculations or a more accurate simulation using LTSpice [36]. Finally, the core EY module calculates the energy yield of the solar cell, accounting for the solar module orientation (rotation and/or tilt) and location. Temperature effects are inherently accounted for using the nominal operating cell temperature (NOCT) model [37]. In this study, we assumed an NOCT value of 48 and derived the insolation on the cell as well as the ambient air temperature from TMY3 data.

## 5.2 Standardized Test Conditions performance comparison

In order to explain the differences in EY across the various thicknesses in the selected organic solar cell, we use EYCalc to evaluate their performance under standard test conditions (see Table 3).

| Thickness [nm] | $J_{sc}$ [mA/cm$^2$] | $V_{oc}$[V] | FF | PCE |
|---|---|---|---|---|
| 100 | 19.8098 | 0.7579 | 0.7038 | 0.1057 |
| 200 | 24.3280 | 0.7582 | 0.6033 | 0.1113 |
| 300 | 28.7523 | 0.7543 | 0.4678 | 0.1015 |

Table 3: EYCalc-based comparison of the performance of the selected organic solar cell across three thicknesses (100 nm, 200 nm, 300 nm) under standard test conditions (STC), highlighting the simulated $J_{sc}$, $V_{oc}$, FF, and the resulting power conversion efficiency (PCE).

# 6 Optimization

To benchmark the performance of our differentiable optimization framework beyond the classical gradient descent shown in the main text, we applied a variety of both gradient-based and gradient-free algorithms to the same two-parameter optimization. For each of the algorithms mentioned below, the same four starting points as the main paper (all combinations of two thickness values (125 nm and 275 nm) and two tilt angles (10° and 50°)) are chosen.

## 6.1 Gradient-free methods

### Nelder-Mead

The Nelder-Mead method is a gradient-free simplex algorithm that optimizes a function by evaluating its value at the vertices of a simplex and iteratively modifying the simplex through reflection, expansion, contraction, or shrinkage. It is robust in low-dimensional spaces and suitable for noisy or non-differentiable objective functions, but typically requires more function evaluations to converge.

### Powell

Powell's method is a derivative-free optimization technique that performs sequential line minimizations along a set of directions. These directions are updated over iterations to form a set

of conjugate directions, allowing the method to efficiently explore the parameter space. Powell's method is effective for smooth functions but can be slower than gradient-based methods when gradient information is available.

## 6.2 Gradient-based methods

### L-BFGS-B

The limited-memory Broyden-Fletcher-Goldfarb-Shanno algorithm, known as L-BFGS [38] is employed here. L-BFGS is a quasi-Newton optimization method that efficiently approximates the inverse Hessian matrix to minimize differentiable functions iteratively. Instead of computing the full Hessian, it uses a limited number of past updates, making it memory efficient. A specific version of L-BFGS referred to as L-BFGS-B is used to include parameter bounds for the optimization, thus keeping the optimal parameter values in reasonable intervals determined in advance by the user. More details of the implementation of the L-BFGS-B algorithm are available in references [39, 40].

### TNC

TNC is a Newton-based optimization algorithm that avoids computing the full Hessian by solving the Newton system approximately using iterative methods. It uses gradient and Hessian-vector products to capture curvature information efficiently. TNC is well-suited for large-scale, smooth optimization problems with bound constraints.

## 6.3 Comparison of the gradient-free and gradient-based methods

Table 4 compares the performance of the gradient-free and gradient-based methods. For each method, the same four starting conditions described in the main manuscript are chosen (all combinations of two thickness values 125 nm and 275 nm and two tilt angles 10° and 50°). All the methods reach comparable maxima, but the gradient-free methods reach these maxima in a significantly higher number of function evaluations, and therefore in more computational time. This highlights the superiority of gradient-based methods that use information about the gradients of the function to guide the optimization process. This effect is expected to be even more pronounced with more complicated optimization tasks involving more than just two input parameters, in which case gradient-free methods might be impractical or even impossible to use.

| Method | Type | Number of Evaluations | Duration [s] |
|---|---|---|---|
| Powell | Gradient-free | 881 | 2803 |
| Nelder-Mead | Gradient-free | 474 | 2221 |
| TNC | Gradient-based | 345 | 1134 |
| L-BFGS-B | Gradient-based | 64 | 283 |
| Gradient Ascent | Gradient-based | 40 | 165 |

Table 4: Comparison of gradient-free and gradient-based optimization method performance, along with the number of evaluations and durations required to reach the maxima. As inferred from the table, gradient-free methods require substantially more function evaluations and computational time. This demonstrates the efficiency advantage of gradient-based optimization, which becomes even more significant as problem dimensionality increases.

## 6.4 Summary of optimizable input parameters

This section introduces the various input parameters involved in the Sol(Di)$^2$T framework, summarized in Table 5. These parameters can either have their value changed directly by the user or by using alternative input files.

| Parameter | Unit | Simulation Module | Notes |
|---|---|---|---|
| Active layer thickness ($d_a$) | nm | Optics / Electrics | Value to be changed directly |
| Active layer permittivity ($\varepsilon_a$) | — | Optics | Input file required |
| Other layer permittivities ($\varepsilon$) | — | Optics | Input file required |
| Other layer thicknesses ($d_i$) | nm | Optics | Value to be changed directly |
| Simulation location | — | Energy Yield | Input file required |
| Tilt angle ($\theta_{\mathrm{tilt}}$) | ° | Energy Yield | Value to be changed directly |
| Rotation angle ($\theta_{\mathrm{rot}}$) | ° | Energy Yield | Value to be changed directly |
| Charge collection efficiency ($\eta_{\mathrm{coll}}$) | — | Energy Yield | Value to be changed directly |
| Nominal operating cell temperature ($T_{\mathrm{NOCT}}$) | °C | Energy Yield | Value to be changed directly |
| Forward barrier height ($\phi_{\mathrm{fb}}$) | eV | Electrics | Value to be changed directly |
| Backward barrier height ($\phi_{\mathrm{bb}}$) | eV | Electrics | Value to be changed directly |
| Bandgap energy ($E_g$) | eV | Electrics | Value to be changed directly |
| Zero-field mobility ($\mu_0$) | $\mathrm{m^2V^{-1}s^{-1}}$ | Electrics | Value to be changed directly |
| Radiative recombination pre-factor ($k_{r0}$) | $\mathrm{m^3s^{-1}}$ | Electrics | Value to be changed directly |

Table 5: Model parameters and input data used in the simulation framework. The simulation module indicates which part of the workflow each parameter is involved in.

# References


[1] Yubo Geng et al. "Impact of crystallinity and grain density on the charge-carrier distribution and transport in organic semiconductors". In: *Organic Electronics* 127 (2024), p. 107006. DOI: https://doi.org/10.1016/j.orgel.2024.107006.

[2] Chris Groves. "Developing understanding of organic photovoltaic devices: kinetic Monte Carlo models of geminate and non-geminate recombination, charge transport and charge extraction". In: *Energy & Environmental Science* 6.11 (2013), p. 3202. DOI: https://doi.org/10.1039/C3EE41621F.

[3] Michael C. Heiber et al. "Impact of tortuosity on charge-carrier transport in organic bulk heterojunction blends". In: *Physical Review Applied* 8.5 (2017), p. 054043. DOI: https://doi.org/10.1103/PhysRevApplied.8.054043.

[4] Rong Wang et al. "Tailoring the nature of interface states in efficient and stable bilayer organic solar cells by a transfer-printing technique". In: *Advanced Materials Interfaces* 9.15 (2022), p. 2200342. DOI: https://doi.org/10.1002/admi.202200342.

[5] Ryan S. Gebhardt et al. "A data-driven identification of morphological features influencing the fill factor and efficiency of organic photovoltaic devices". In: *Computational Materials Science* 129 (2017), p. 220. DOI: https://doi.org/10.1016/j.commatsci.2016.12.020.

[6] Olga Wodo et al. "Quantifying organic solar cell morphology: a computational study of three-dimensional maps". In: *Energy & Environmental Science* 6.10 (2013), p. 3060. DOI: https://doi.org/10.1039/c3ee41224e.

[7] Benedikt Zerulla et al. "A Multi-Scale Approach for Modeling the Optical Response of Molecular Materials Inside Cavities". In: *Advanced Materials* 34.21 (2022), p. 2200350. DOI: https://doi.org/10.1002/adma.202200350. eprint: https://onlinelibrary.wiley.com/doi/pdf/10.1002/adma.202200350. URL: https://onlinelibrary.wiley.com/doi/abs/10.1002/adma.202200350.

[8] Benedikt Zerulla et al. "A T-Matrix Based Approach to Homogenize Artificial Materials". In: *Advanced Optical Materials* 11.3 (2023), p. 2201564. DOI: https://doi.org/10.1002/adom.202201564. eprint: https://onlinelibrary.wiley.com/doi/pdf/10.1002/adom.202201564. URL: https://onlinelibrary.wiley.com/doi/abs/10.1002/adom.202201564.

[9] *TURBOMOLE V7.8 2023, a development of University of Karlsruhe and Forschungszentrum Karlsruhe GmbH, 1989-2007, TURBOMOLE GmbH, since 2007.*

[10] Yannick J. Franzke et al. "TURBOMOLE: Today and Tomorrow". In: *Journal of Chemical Theory and Computation* 19.20 (2023), pp. 6859–6890.

[11] Carlo Adamo and Vincenzo Barone. "Toward Reliable Density Functional Methods without Adjustable Parameters: The PBE0 Model". In: *The Journal of Chemical Physics* 110.13 (1999), pp. 6158–6170.

[12] Matthias Ernzerhof and Gustavo E. Scuseria. "Assessment of the Perdew–Burke–Ernzerhof Exchange-Correlation Functional". In: *The Journal of Chemical Physics* 110.11 (1999), pp. 5029–5036.

[13] Florian Weigend and Reinhart Ahlrichs. “Balanced Basis Sets of Split Valence, Triple Zeta Valence and Quadruple Zeta Valence Quality for H to Rn: Design and Assessment of Accuracy”. In: *Phys. Chem. Chem. Phys.* 7.18 (2005), pp. 3297–3305.

[14] K Eichkorn et al. “Auxiliary Basis Sets to Approximate Coulomb Potentials (Chem. Phys. Letters 240 (1995) 283-290)”. In: *Chemical Physics Letters* 242.6 (1995), pp. 652–660.

[15] Karin Eichkorn et al. “Auxiliary Basis Sets for Main Row Atoms and Transition Metals and Their Use to Approximate Coulomb Potentials”. In: *Theor Chem Acta* 97.1 (1997), pp. 119–124.

[16] Florian Weigend. “Accurate Coulomb-fitting Basis Sets for H to Rn”. In: *Phys. Chem. Chem. Phys.* 8.9 (2006), pp. 1057–1065.

[17] Takeshi Yanai, David P Tew, and Nicholas C Handy. “A new hybrid exchange–correlation functional using the Coulomb-attenuating method (CAM-B3LYP)”. In: *Chemical Physics Letters* 393.1 (2004), pp. 51–57. ISSN: 0009-2614. DOI: https://doi.org/10.1016/j.cplett.2004.06.011. URL: https://www.sciencedirect.com/science/article/pii/S0009261404008620.

[18] Jianmin Tao et al. “Climbing the Density Functional Ladder: Nonempirical Meta–Generalized Gradient Approximation Designed for Molecules and Solids”. In: *Phys. Rev. Lett.* 91 (14 Sept. 2003), p. 146401. DOI: 10.1103/PhysRevLett.91.146401.

[19] Viktor N. Staroverov et al. “Comparative assessment of a new nonempirical density functional: Molecules and hydrogen-bonded complexes”. In: *The Journal of Chemical Physics* 119.23 (Dec. 2003), pp. 12129–12137. ISSN: 0021-9606. DOI: 10.1063/1.1626543.

[20] Viktor N. Staroverov et al. “Erratum: “Comparative assessment of a new nonempirical density functional: Molecules and hydrogen-bonded complexes” [J. Chem. Phys. 119, 12129 (2003)]”. In: *The Journal of Chemical Physics* 121.22 (Dec. 2004), pp. 11507–11507. ISSN: 0021-9606. DOI: 10.1063/1.1795692.

[21] Reinhart Ahlrichs. “Efficient evaluation of three-center two-electron integrals over Gaussian functions”. In: *Phys. Chem. Chem. Phys.* 6 (2004), pp. 5119–5121.

[22] Marek Sierka, Annika Hogekamp, and Reinhart Ahlrichs. “Fast Evaluation of the Coulomb Potential for Electron Densities Using Multipole Accelerated Resolution of Identity Approximation”. In: *The Journal of Chemical Physics* 118.20 (2003), pp. 9136–9148.

[23] Christof Holzer. “An improved seminumerical Coulomb and exchange algorithm for properties and excited states in modern density functional theory”. In: *The Journal of Chemical Physics* 153.18 (2020), p. 184115.

[24] Weigang Zhu et al. “Crystallography, Morphology, Electronic Structure, and Transport in Non-Fullerene/Non-Indacenodithienothiophene Polymer:Y6 Solar Cells”. In: *Journal of the American Chemical Society* 142.34 (2020). PMID: 32698577, pp. 14532–14547. DOI: 10.1021/jacs.0c05560.

[25] Jun Yuan et al. “Single-Junction Organic Solar Cell with over 15% Efficiency Using Fused-Ring Acceptor with Electron-Deficient Core”. In: *Joule* 3.4 (2019), pp. 1140–1151. ISSN: 2542-4351. DOI: https://doi.org/10.1016/j.joule.2019.01.004.

[26] Ivan Fernandez-Corbaton et al. “Computation of electromagnetic properties of molecular ensembles”. In: *ChemPhysChem* 21 (2020), pp. 878–887.

[27] Dominik Beutel, Ivan Fernandez-Corbaton, and Carsten Rockstuhl. “treams – a T-matrix-based scattering code for nanophotonics”. In: *Computer Physics Communications* 297 (2024), p. 109076. ISSN: 0010-4655. DOI: https://doi.org/10.1016/j.cpc.2023.109076. URL: https://www.sciencedirect.com/science/article/pii/S0010465523004216.

[28] Wei Li et al. “Organic solar cells with near-unity charge generation yield”. In: *Energy Environ. Sci.* 14 (12 2021), 6484–6493". DOI: 10.1039/D1EE01367J. URL: http://dx.doi.org/10.1039/D1EE01367J.

[29] Heng Zhao et al. “Hot Hydrocarbon-Solvent Slot-Die Coating Enables High-Efficiency Organic Solar Cells with Temperature-Dependent Aggregation Behavior”. In: *Advanced Materials* 32.39 (2020), p. 2002302. DOI: https://doi.org/10.1002/adma.202002302. URL: https://advanced.onlinelibrary.wiley.com/doi/abs/10.1002/adma.202002302.

[30] Floris Laporte. *SAX: S-Matrices with Autograd and XLA - a scatter parameter circuit simulator and optimizer for the frequency domain based on JAX.* Version 0.14.1. 2024. URL: https://flaport.github.io/sax/.

[31] Miguel Alexandre et al. "SCATMM: Easy-to-Use Graphical User Interface for Light Propagation in Arbitrary Multilayers." In: *Journal of Open Research Software* 12:11 (2024). DOI: https://doi.org/10.5334/jors.511.

[32] Maria Saladina and Carsten Deibel. "Transport resistance strikes back: unveiling its impact on fill factor losses in organic solar cells". In: *Reports on Progress in Physics* (2024).

[33] Nurlan Tokmoldin et al. "Extraordinarily long diffusion length in PM6: Y6 organic solar cells". In: *Journal of Materials Chemistry A* 8.16 (2020), pp. 7854–7860.

[34] Raphael Schmager et al. *EYcalc - Energy yield calculator for multi- junction solar modules with realistic irradiance data and textured interfaces*. Version v1.0. May 2021. DOI: 10.5281/zenodo.4696257. URL: https://doi.org/10.5281/zenodo.4696257.

[35] Simeon C. Baker-Finch and Keith R. McIntosh. "Reflection of normally incident light from silicon solar cells with pyramidal texture". In: *Progress in Photovoltaics: Research and Applications* 19.4 (Oct. 2010), pp. 406–416. ISSN: 1099-159X. DOI: 10.1002/pip.1050. URL: http://dx.doi.org/10.1002/pip.1050.

[36] *Analog Devices, Inc. LTSpice*. https://www.analog.com/en/design-center/design-tools-and-calculators/ltspice-simulator.html. [Accessed January 2025].

[37] M.C. Alonso García and J.L. Balenzategui. "Estimation of photovoltaic module yearly temperature and performance based on Nominal Operation Cell Temperature calculations". In: *Renewable Energy* 29.12 (2004), pp. 1997–2010. URL: https://EconPapers.repec.org/RePEc:eee:renene:v:29:y:2004:i:12:p:1997-2010.

[38] Dong C. Liu and Jorge Nocedal. "On the limited memory BFGS method for large scale optimization". In: *Mathematical Programming* 45.1 (Aug. 1989), pp. 503–528. ISSN: 1436-4646. DOI: 10.1007/BF01589116. URL: https://doi.org/10.1007/BF01589116.

[39] Richard H Byrd et al. "A limited memory algorithm for bound constrained optimization". In: *SIAM Journal on scientific computing* 16.5 (1995), pp. 1190–1208.

[40] Ciyou Zhu et al. "Algorithm 778: L-BFGS-B: Fortran subroutines for large-scale bound-constrained optimization". In: *ACM Transactions on mathematical software (TOMS)* 23.4 (1997), pp. 550–560.
